# Supplementary material for: PhyPlan: Generalizable and Rapid Physical Task Planning with Physics Informed Skill Networks for Robot Manipulators
Source: arXiv:2406.00001 source file (2024-04-22)
Supplement: Supplementary file 1 [file appendix.tex]

\noindent This section includes the details of network architecture, perception methodology and the algorithm of Physics-informed rollouts with a visual description of the working of the algorithm. We also describe Prompting strategy adopted to evaluate Physical Reasoning in LLM Baseline.

\subsection{Skill Learning}  

In Table \ref{tab:neural_network}, we present a comprehensive overview of the Fully Connected Neural Network architecture implemented within various Physics-Informed Skill Networks. These networks integrate neural network models and physics-based governing equations specific to each skill. Additionally, Table \ref{table:Skill-Table} lists the inputs, outputs, and governing equations pertinent to each skill network. In this context, the subscript $init$ signifies the initial value of a physical parameter, and $t_{query}$ denotes the time instance for which the output quantity is required. The terms $v_{hor}$ and $v_{ver}$ are used to represent planar and vertical velocities, respectively, with the latter directed towards gravity (g). Key parameters such as the angle $\theta$ of a wedge in the bouncing skill and the masses $m_{1}$ and $m_{2}$ of colliding objects in the hitting skill are also inputs to their respective skill networks. Note that the skills like Bouncing and Hitting are exclusively trained through data-driven approaches, and hence, they do not incorporate any governing differential equations.

\begin{multicols}{2}
    \begin{figure}[H]
        \centering
        \subfloat[]{\includegraphics[width=0.3\linewidth]{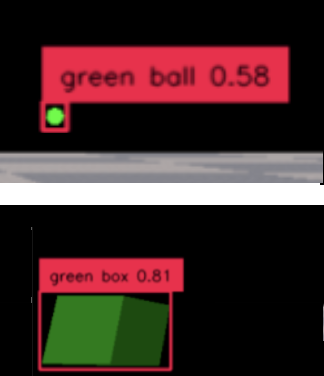}}
        \subfloat[]{\includegraphics[width=0.3\linewidth]{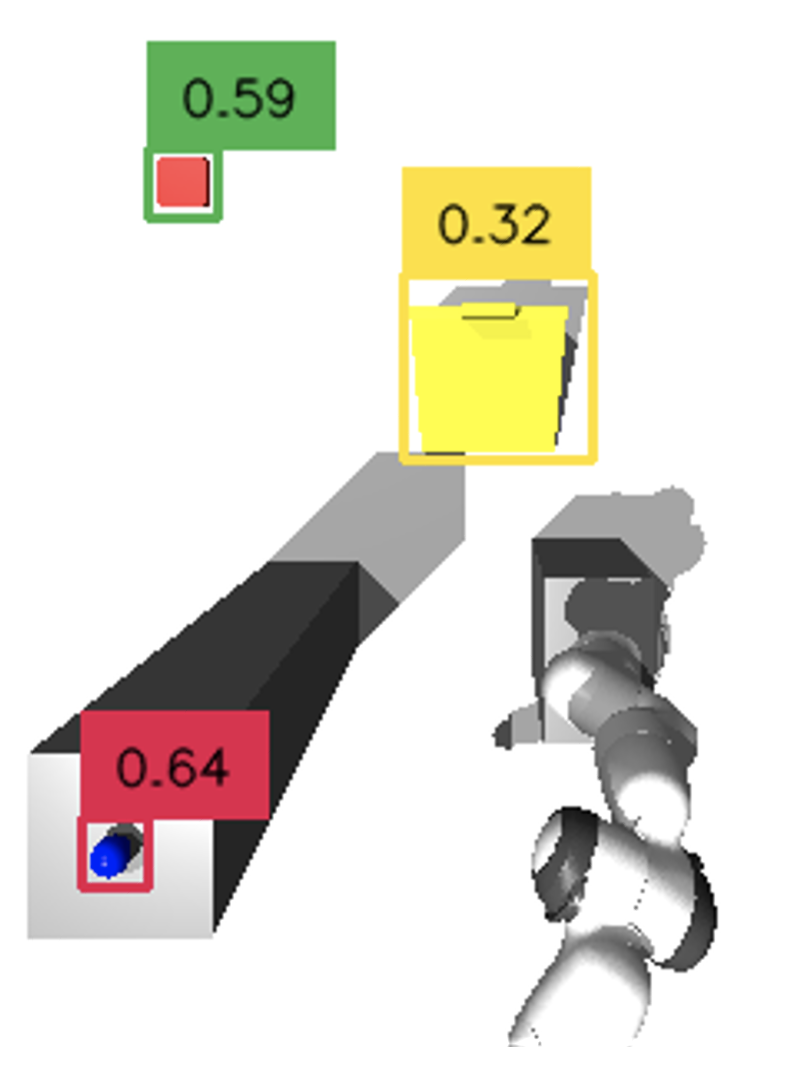}}
        \subfloat[]{\includegraphics[width=0.3\linewidth]{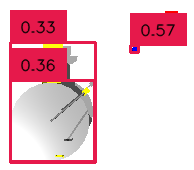}}
        \vspace{3mm}
        \caption{\footnotesize Showing perception-based bounding box detection of a) ball being thrown and sliding box, to learn skills, b) wedge and goal in bounce task and c) goal in bridge task, for task inference}
        \label{fig:mcts-exp-perception}
    \end{figure}
    
    \begin{table}[H]
        \small
        \centering
        % \begin{tabular}{|l|l|}
        \begin{tabular}{@{}ll@{}}
        \toprule
        \textbf{Parameter} & \textbf{Value} \\
        \midrule
        Number of Layers & 10 (1 input, 8 hidden, 1 output) \\
        Input Layer & Initial condition (pos, vel), $t_{query}$\\
        Output Layer & pos, vel at $t_{query}$\\
        Neurons in Hidden Layers & 40 \\
        Activation Function (Hidden) & Tanh \\
        Activation Function (Output) & None \\
        Optimizer Type & L-BFGS \\
        Learning Rate & 0.01 \\
        Maximum Training Cycles & 6400 \\
        Initialization & Xavier/Glorot Normal \\
        \bottomrule
        \end{tabular}
        \caption{\footnotesize General Neural Network Configuration used in different Physics-Informed Skill Networks}
        \label{tab:neural_network}
    \end{table}
\end{multicols}

\begin{table}[H]
    \centering
     % Adjust the cell spacing
    \resizebox{\textwidth}{!}{%
    \begin{tabular}{||l|l|l|l|l|l||}
        \toprule
        Skill & Swinging & Sliding & Throwing & Bouncing & Hitting \\[2pt]
        \midrule
        Input & $(\theta_{init}, t_{query})$ & $(v_{init}, t_{query})$ & $(v_{{hor}_{init}}, v_{{ver}_{init}}, t_{query})$ & $(e,\theta, v_{{ver}_{init}}, v_{{hor}_{init}})$ & $(m_{1},m_{2}, v_{init})$ \\[2pt]
        \hline
        Output & $(\theta_{query}, \omega_{query})$ & $(x_{query}, v_{query})$ & $(v_{{ver}_{query}}, y_{query}, x_{query})$ & $(v_{{ver}_{query}}, v_{{hor}_{query}})$ &  $v_{query}$ \\[2pt]
        \hline
        ODE & $\frac{d^2\theta}{dt^2} + \frac{g * sin(\theta)}{l} = 0,$ &  $\frac{d^2x}{dt^2} + \mu g = 0,$  & $\frac{v_{{ver}_{init}}}{dt} + g = 0, \frac{d^2y}{d^2t} + g = 0,$  & None &  None \\[2pt]
        
        & $\frac{d\omega}{dt} + \frac{g * sin(\theta)}{l} = 0$  & $ \frac{dv}{dt} + \mu g = 0$ & $ \frac{dx}{dt} - v_{{hor}_{init}} = 0$ &  & \\[2pt]
        \bottomrule
    \end{tabular}
    }
    \caption{\textbf{Physics Informed Skill Networks.} Showing the input, output, and ODE used to train different skill networks.}
    \label{table:Skill-Table}
    % \vspace{2mm}
\end{table}

% \begin{figure*}[h]
%     \centering
%     \subfloat[Throwing Skill]{\includegraphics[width=0.33\linewidth]{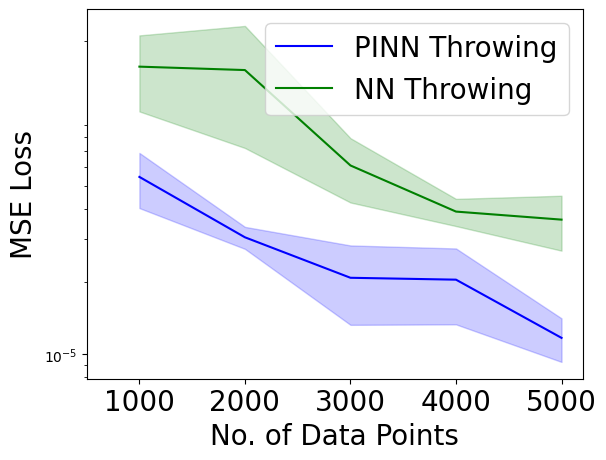}}
%     \subfloat[Sliding Skill]{\includegraphics[width=0.33\linewidth]{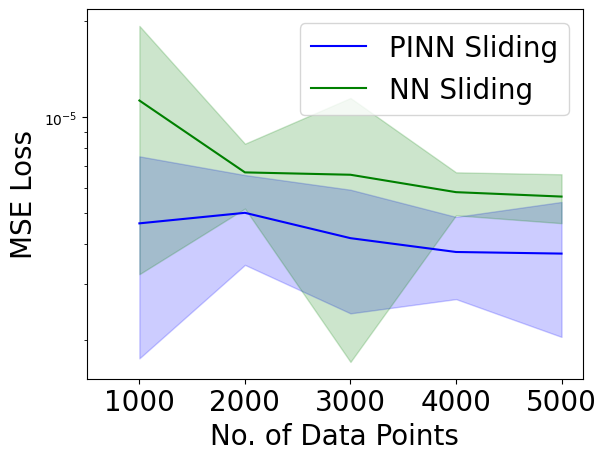}}
%     \subfloat[Swinging Skill]{\includegraphics[width=0.33\linewidth]{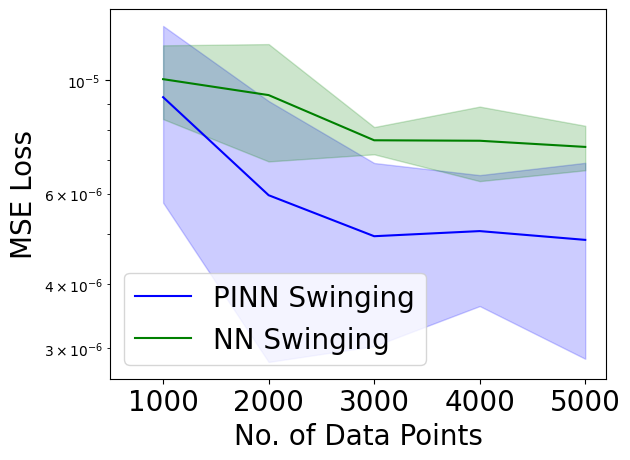}}
%     \vspace{2mm}
%     \caption{PINN displays superior data efficiency over NN, highlighted by lower MSE loss in various initial settings.}
%     \label{fig:data-eff}
%     % \vspace{3mm}
% \end{figure*}

Figure \ref{fig:mcts-exp-perception} illustrates the object detection strategy employed in our Perception-based pipeline. Here, environmental scene images are processed using the 'Segment Anything' \cite{kirillov2023segment} and 'Grounding Dino' \cite{liu2023grounding} models, which efficaciously detect targeted objects within a defined confidence. 

% Figure \ref{fig:data-eff} underscores the data efficiency of our employed Physics-Informed Neural Network in modeling physical skills. The PINN models exhibit lower Mean Squared Error (MSE) loss on the validation dataset with a relatively small number of training data points, compared to conventional Neural Network models.

\subsection{PINN based Simulator}  

In Section $4$ of the main paper, we delineate the intricacies of the algorithm employed in our study. Broadly, the \emph{Adaptive Physical Task Reasoning} serves as the encompassing algorithm that invokes the \emph{Physics-Informed MCTS} to acquire a nuanced reward model and adapt to the dynamic environment. The \emph{Physics-Informed MCTS} performs semantic rollouts via the \emph{PINN-Rollout} to approximate the value of actions, subsequently expanding the MCTS tree as per the insights gained.

\begin{figure*}[]
    \centering
    \begin{subfigure}[t]{0.245\linewidth}
        \includegraphics[width=\linewidth, height=0.855\linewidth]{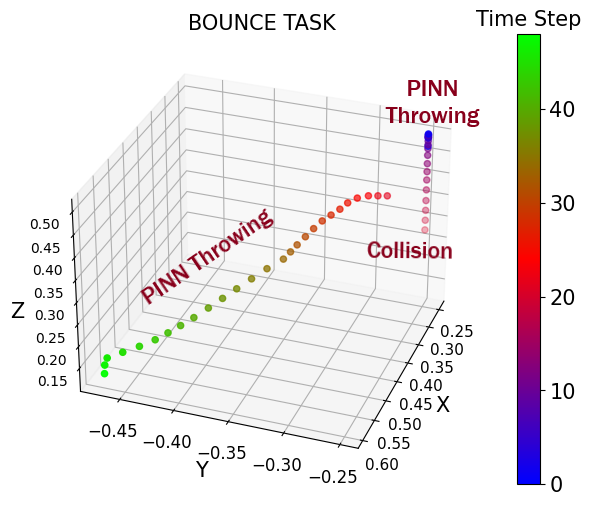}
        \caption{}
        \label{fig:bounce_chain_0.5}
    \end{subfigure}
    \hfill  
    \begin{subfigure}[t]{0.245\linewidth}
        \includegraphics[width=\linewidth, height=0.855\linewidth]{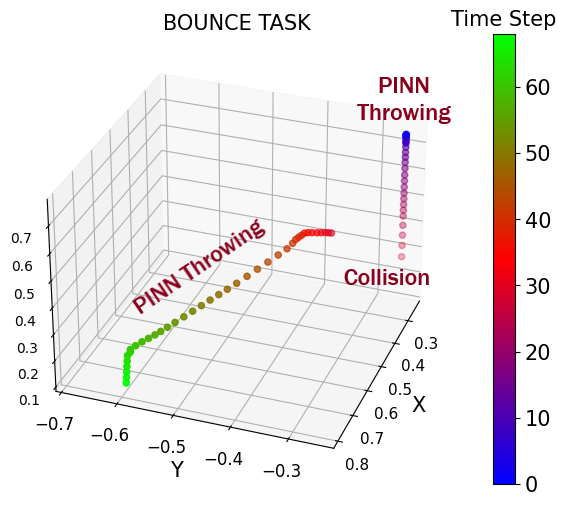}
        \caption{}
        \label{fig:bounce_chain_0.75}
    \end{subfigure}
    \hfill 
    \begin{subfigure}[t]{0.245\linewidth}
        \includegraphics[width=\linewidth, height=0.855\linewidth]{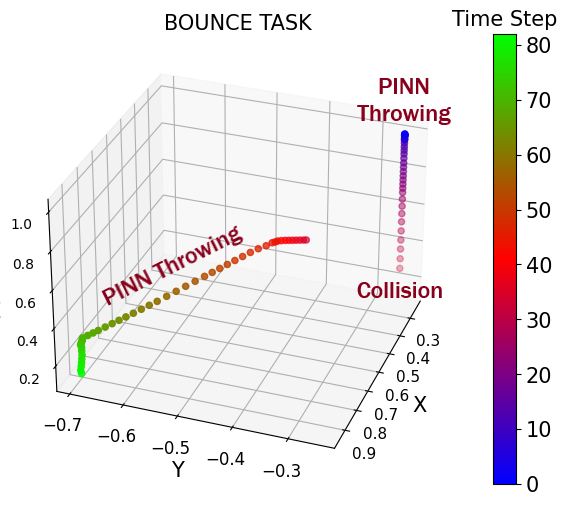}
        \caption{}
        \label{fig:bounce_chain_1}
    \end{subfigure}
    \hfill 
    \begin{subfigure}[t]{0.245\linewidth}
        \includegraphics[width=\linewidth, height=0.855\linewidth]{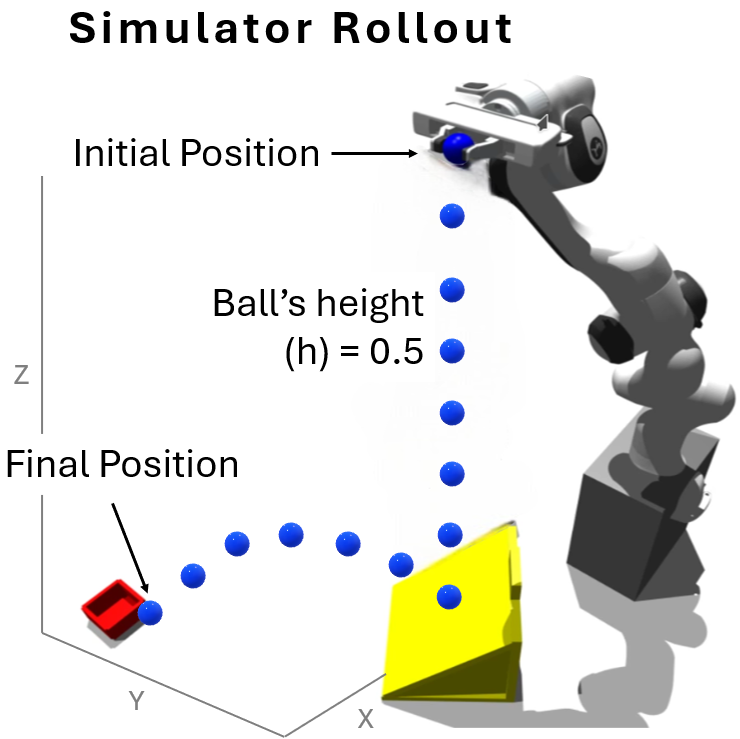}
        \caption{}
        \label{fig:simulator_rollout}
    \end{subfigure}
    
\caption{\footnotesize \textbf{Rapid Trajectory Prediction using PINN\_Rollouts.} Simulated trajectory of the ball interacting with a wedge obtained by composing predictions of Physics-Informed Skill Networks for each skill (throwing, collision, and projectile motion in sequence). The agent varies the initial drop height (here a)0.5, b)0.75, and c)1.0) and uses PINN\_Rollout to determine the final resting position of the ball to evaluate the reward. Such fast trajectory simulations are used within the MCTS planner. The trajectory with the best reward is eventually employed to be simulated in the real world represented by d)}

    \label{fig:bounce_chain}
\end{figure*}

Figure \ref{fig:bounce_chain} illustrates PINN\_Rollout in action for the bounce task. It shows the PINN-predicted trajectory of the ball for various initial heights tested by the agent. Notably, the ball's final resting position corresponds to an increasing trend with respect to the initial drop height. Specifically, the ball's terminal position for an initial height of $1.0$ exceeds that for $0.75$, which, in turn, surpasses the final position for an initial height of $0.5$. The PINN model demonstrates a notable capability to emulate the physical trajectory of the ball, aligning with the principles of physics governing the ball's motion.

\subsection{LLM Baseline - Prompt Details}

\begin{table}[H]
\centering
\begin{tabular}{|p{\textwidth}|}
\hline
\\[0.5pt]
\emph{\textbf{Initial Prompt (Task Description):}}
\\[5pt]
\hline
\\[1pt]
There is a robot and a goal located at \texttt{goal\_pos} outside the direct reach of the robot. There is a ball that needs to reach the goal. The environment has a fixed pillar over which the ball rests, and a pendulum hanging over the ball that the robot can orient to hit the ball to throw it to the goal. The robot can orient the pendulum along any vertical plane and choose to drop the pendulum from any angle from the vertical axis. When hit with a pendulum, the puck projectiles and lands far away on the ground.\\
Sanity check 1: How does the plane of the pendulum affect the puck's position with respect to the goal?\\
Sanity check 2: How does the drop angle of the pendulum affect the puck's position with respect to the goal?\\
\\[1pt]
\hline
\\[0.5pt]
\emph{\textbf{Initial Response (Sanity Check):}}
\\[5pt]
\hline
\\[0.5pt]
\includegraphics[width=\linewidth]{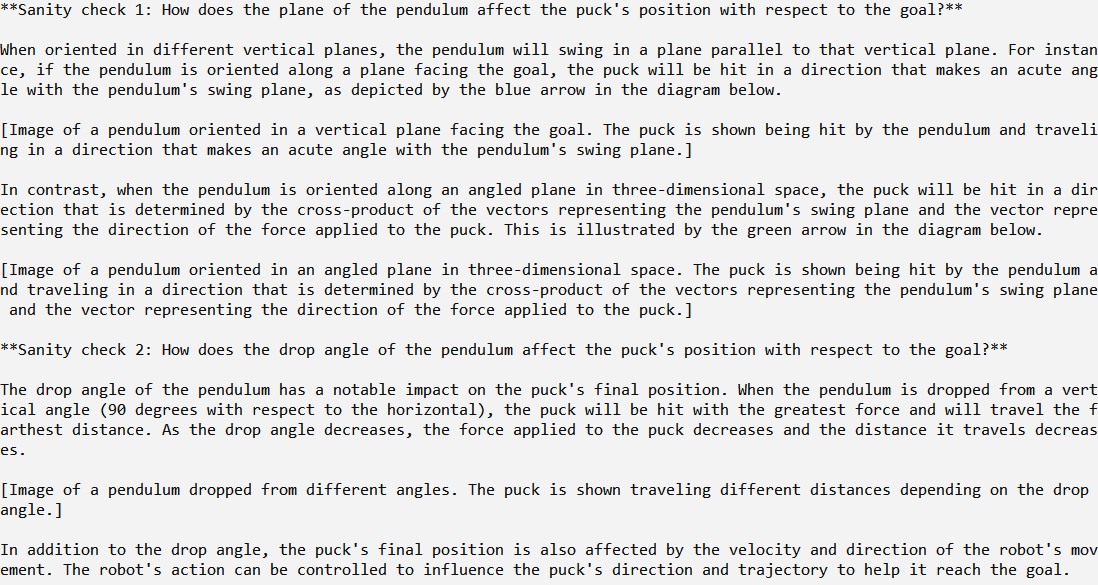}\\
\\[1pt]
\hline
\end{tabular}
\caption{\footnotesize Prompt describing task for evaluating Physical Reasoning Abilities of LLM Baseline for the Launch Task. LLM's response reflects the task image inferred from the prompt.}
\label{table:launch_task}
\end{table}

\begin{table}[H]
\centering
\begin{tabular}{|p{\textwidth}|}
\hline
\\[0.5pt]
\emph{\textbf{Feedback Prompt:}} 
\\[5pt]
\hline
\\[1pt]
\begin{minipage}[c]{0.58\textwidth}
In one line, give the numerical values of the angle to orient the pendulum's plane and the angle to drop the pendulum from (both in decimal radians). The bound for plane orientation angle is \texttt{{bnds[0][0]}, {bnds[0][1]}} and that for drop angle with vertical axis is \texttt{{bnds[1][0]}, {bnds[1][1]}}. I will tell you where the ball landed, and you should modify your answer accordingly till the ball reaches the goal. I have marked the ground into two halves. The goal lies in one half, and the robot and the wedge are at the centre. Throughout the conversation, remember that my response would be one of these:
\begin{enumerate}
    \item The ball lands in the half not containing the goal, I'd say 'WRONG HALF'.
    \item The ball lands in the correct half but left of the goal, I'd say 'LEFT by \textless{}horizontal distance between ball and goal\textgreater{}'.
    \item The ball lands in the correct half but the right of the goal, I'd say 'RIGHT by \textless{}horizontal distance between ball and goal\textgreater{}'.
    \item The ball lands in the correct half and in line but overshot the goal, I'd say 'OVERSHOT by \textless{}horizontal distance between ball and goal\textgreater{}'.
    \item The ball lands in the correct half and in line but falls short of the goal; I'd say 'FELL SHORT by \textless{}horizontal distance between ball and goal\textgreater{}'.
    \item Finally, the ball successfully landed in the goal; I'd say 'GOAL'.
\end{enumerate}
Note: In your response, do not write anything else except the (pendulum's plane and drop angles) pair. Send in tuple FORMAT: (angle 1, angle 2). Do not emphasise the answer; just return plain text. Let's begin with an initial guess!\\
\end{minipage}
\hfill
\begin{minipage}[c]{0.4\textwidth}
    \includegraphics[width=\textwidth]{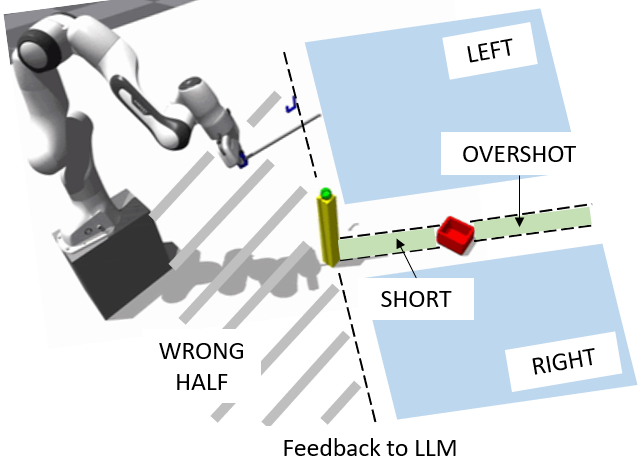}
\end{minipage}
\\[1pt]
\hline
\\[0.5pt]
\emph{\textbf{Response to successive feedbacks from the execution environment:}}
\\[5pt]
\hline
\\[0.5pt]
\includegraphics[width=0.7\linewidth]{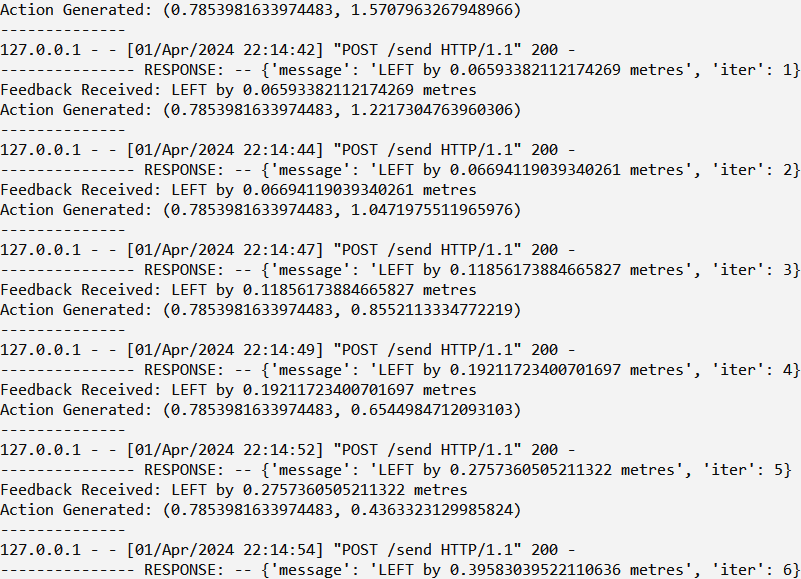}\\
\\[1pt]
\hline
\end{tabular}
\caption{\footnotesize Rollout of LLM generating action and receiving feedback from the execution environment. The LLM starts well, as the distance between the ball and the goal is low but successively diverges after receiving the feedback.}
\label{table:launch_task}
\end{table}

We examined the capabilities of Large Language Models (LLMs) in performing tasks requiring physical reasoning, with a focus on Google's Gemini-Pro model \cite{google2023gemini}. Our approach entailed presenting the LLM with a series of tasks set within a simulated environment, for which it was required to generate action sequences. These actions were then executed in the environment, and feedback regarding the outcome, specifically, the position of a ball or puck relative to a target, was provided to the LLM for refinement of subsequent actions.
Our methodology comprised two primary steps: an initial prompt detailing the task and environment setting, a feedback prompt relaying the actions' outcomes, and information about the environment's dynamics and the underlying reward model. This process allowed the LLM to adjust its strategies based on the feedback, simulating a trial-and-error learning mechanism. An example of the prompting strategy used for the "Launch Task" is depicted in Table \ref{table:launch_task}, which outlines the structure of the initial and feedback prompts. The complete details of the prompts used for each task are available on the project website:  \textcolor{blue}{\href{https://phyplan.github.io}{https://phyplan.github.io}}.
